# Supplementary material for: Comparison of Algorithms for Simple Stochastic Games (Full Version)
Source: arXiv:2008.09465 source file (2020-08-25)
Supplement: Supplementary file 1 [file 3_3_SI.tex]

In contrast to value iteration, the approach of strategy iteration~\cite{HK66} does not compute a sequence of value-vectors, but instead a sequence of strategies.
Starting from an arbitrary strategy of Maximizer, we repeatedly compute the best response of Minimizer and then greedily improve Maximizer's strategy. The resulting sequence of Maximizer strategies is monotonic and converges to the optimal strategy~\cite[Theorem 3]{CAH13}.
The pseudocode for strategy iteration is given in Algorithm \ref{alg:si}.

Note that in non-stopping games the initial Maximizer strategy cannot be completely arbitrary, but it has to be \emph{proper}, i.e. ensure that either a target or a sink state is reached almost surely; it must not stay in some end component, as otherwise the algorithm might not converge to the optimum due to problems similar to those described in Example \ref{ex:ubNoConvergeVI}.
In Algorithm \ref{alg:si}, we use the construction of the \emph{attractor strategy}~\cite[Section 5.3]{CAH13} to ensure that our initial guess is a proper strategy (Line \ref{line:si_attractor}). It works by a backwards breadth first search from the target and sink states. 
A state discovered in the $i$-th iteration of the search has to choose some action that reaches a state discovered in the $(i-1)$-th iteration with positive probability (such a state exists by construction).

When a Maximizer strategy is fixed, the main loop of Algorithm \ref{alg:si} solves the induced MDP $\game[\straa]$ (Line \ref{line:si_mdp}). 
It does not remember the Minimizer strategy, but only uses the computed value estimates $\lb$ to greedily update Maximizer's strategy (Line \ref{line:si_update}); note that here $\lb(\state,\action)$ is again computed from $\lb(\state)$ as in Equation \ref{eq:Vsa}.

The algorithm stops when the Maximizer strategy does not change any more in one iteration. We can then compute the values and the corresponding Minimizer strategy by solving the induced MDP $\game[\straa]$.

\begin{algorithm}[htbp]

	\caption{Strategy iteration}\label{alg:si}
	\begin{algorithmic}[1]
		\Procedure{SI}{}
		\State $\straa' \gets$ arbitrary Maximizer \emph{attractor strategy} \label{line:si_attractor}
		\Repeat
			\State $\straa \gets \straa'$
			\For {$\state \in \states$}
				\State $\lb \gets \inf_{\strab} \pr_{s}^{\straa,\strab}(\Diamond \fstates)$ \label{line:si_mdp}
			\EndFor
			\For {$\state \in \states<\Box>$}
				\State $\straa'(\state) \gets \argmax_{\action \in \Av(\state)} \lb(\state,\action) $ \label{line:si_update}
			\EndFor
		\Until{$\straa = \straa'$}
		\EndProcedure
	\end{algorithmic}
\end{algorithm}

We now propose several optimizations, inspired by \cite{KM17}, of the strategy iteration algorithm to reduce its runtime.

\subsection{Initial strategy} \label{sec:si_init}

Choosing a good initial strategy can speed up the algorithm, as it reduces the number of iterations of the main loop and thus the runtime.
The only necessary requirement for the initial strategy is that it is proper, i.e. it ensures that either target or sink states are reached almost surely.
Using an attractor strategy is one way to ensure this; however, there are multiple attractor strategies, and we can choose any of them. Additionally, an attractor strategy might be highly suboptimal, as it might choose an action leading to a sink state in the backwards DFS, even if the state actually can reach the target (via a longer path).

Hence, we suggest to use any pre-existing knowledge about the model to choose a promising initial strategy, and then verify that it is proper. If it is not, we switch those choices that are necessary to make it so.

Practically, we chose to run unguaranteed value iteration first in order to get some estimates of the values. We use those estimates to guess the initial strategy, ensure that it is proper, and then find the optimal strategy from this starting point.
Note that this is similar in spirit to the idea of optimistic value iteration~\cite{OVI}: utilize value iteration ability to usually deliver tight lower bounds and then verify them. 
But, while value iteration is only a semi-algorithm and might have to attempt verifying the lower bounds repeatedly, strategy iteration certainly converges to the optimal strategy.

\subsection{Opponent strategy}
We can tune the MDP solution method that is used to compute the opponent strategy in Line \ref{line:si_mdp} of algorithm \ref{alg:si}.
Similarly to the layout of this paper, one can consider three variants: Value iteration, strategy iteration or linear programming (LP). 
We need to ensure that we fix the new choices of Maximizer correctly; for this, we do not need the precise solution of the induced MDP, but it suffices to know that an action is better than all others. So for bounded value iteration, it suffices to check that the lower bound of one action is larger than the upper bound of all others and we need not run until a certain precision is reached in all states.
Of course, using the precise solution methods SI and LP is also possible.

As discussed in Section \ref{sec:si_init} for SI, good initial choices can speed things up even further; the same is possible for VI and LP.
We can use the estimate $\lb$ of the previous iteration as a lower bound for the values when solving the induced MDP.

\subsection{MEC decomposition / Topological SI}
Cite \cite[Algorithm 3]{KM17} and https://arxiv.org/abs/1401.3910 and ensuring reliability of model checker TVI chapter.

(compare to topological VI, is the name ok? see ensuring the reliability paper, talks about topological VI)

In order to reduce the number of iteration necessary until convergence, we may want to look at partitions of the complete game, which we can independently solve and then rejoin. One obvious candidate for such a partitioning are SECs, described in \cite{techreport}, as the value in all the states of a SEC is the same. However, one quickly realizes that the problem of partitioning the game into SECs is at least as complicated as solving reachability itself. Another promising partitioning is in MECs, as those are much easier to compute, at the expense of worse properties.

\begin{definition}[MEC]
A non-empty set $T \subset \states$ of states is an end component (EC) if there is a non-empty set $B \subset \bigcap\limits_{\state \in T} Av(\state)$ of actions such that:
\begin{enumerate}
\item for each $\state \in T, a \in B \cap Av(\state)$ we do not have $(\state, a)$ exits $T$,
\item for each $\state, \state' \in T$ there is a finite path $w = \state a_0 ...a_n\state' \in (T \times B)* \times T$, i.e. the path stays inside T and only uses actions in $B$.
\end{enumerate}
An end component $T$ is a maximal end component (MEC) if there is no other end component $T'$ such that $T \subset T'$.
\end{definition}

\textcolor{red}{TODO: a few words about the useful properties of MECs and why we chose them.} 

One downside of MECs is that they cannot be topologically sorted with respect to all the edges. Even if two MECs $i$ and $j$ are no accessible \textcolor{red}{(accessible means that there is a path from one to the other)} from one another with the actions $B_i$ and $B_j$, they could be when considering the entire set of actions $A$. \textcolor{red}{TODO: Add figure similar to Con93, Page 5.}

\begin{algorithm}[htbp]

	\caption{Reachability on MEC decomposition}\label{alg:mec}
	\begin{algorithmic}[1]
		\Procedure{MEC SI}{precision $\epsilon>0$}
		\State $M = \{M_1, ... , M_n\} = $ MEC decomposition
		\State sort $M$ by depth-first-search post-order traversal
		\For {$M_i \in M$} 
		\State $M_i' = $ the set of all states accessible from $M_i$
		\State Solve the SG where only $M_i'$ are the unknown states \Comment{\textcolor{red}{Need better way to write this}}
		\State Update reachability probs in original SG
		\EndFor
		\State $N = \bigcup\limits_{i=1}^{n} M_i$ \Comment{States not part of any MEC}
		\State Solve the SG where only $N$ are the unknown states
		\State Update reachability probs in original SG
		\EndProcedure
	\end{algorithmic}
\end{algorithm}

A \textcolor{red}{cough}, formal, \textcolor{red}{cough}, definition of SI on the MEC decomposition of a SG is given in Algorithm \ref{alg:mec}. After computing the MEC decomposition in line 2, the components are sorted by the depth-first-search post order traversal. Note that after this step, the $n$ components are not necessarily topologically sorted. The for-loop in lines 4-7 processes each MEC $M_i$. First we expand it to contain all accessible states from $M_i$. This is important, as we only solve for the states in $M_i'$. The computations are done on the limited game induced by the states in $M_1', ...,M_i'$. If the game contained paths from $M_i$ to other states outside of the limited game, we would not have definitive results for $M_i$ and would need to recompute the values once states in $M_i' \setminus M_i$ have been added \textcolor{red}{I hope this is clear enough, can't find a better way to phrase it}. Lastly, we update the corresponding values in the original SG. In lines 8-10 we do the same three steps for the states outside any MEC.

It must be noted that we do not improve the worst case performance of the algorithm, because in a game like the one in Figure \textcolor{red}{Con93, Page 5} we essentially solve the entire SG in a single run. It also adds significant overhead for computing the MEC decomposition, which is not efficiently implemented in some tools. \textcolor{red}{TODO: Maybe include some theoretical runtime bounds.} As a result, solving the SG on the MEC decomposition may only offer improvements in the average performance.
